# Supplementary material for: Generalizing DP-SGD with Shuffling and Batch Clipping
Source: arXiv:2212.05796 source file (2023-07-25)
Supplement: Supplementary file 1 [file appendix.tex]

%%%% synchoronous FL Hybrid Batch clipping algorithm %%%%%%
\begin{algorithm}[!ht]
\caption{Hybrid Batch Clipping DPSGD for synchoronous Federated Learning setting}
\label{alg:fed_batch_FL_DPs}
\begin{algorithmic}[1]
%\Procedure{LocalSGDwithDP}{$d,C,s,\sigma,T$}
\Procedure{Federated\_Hybrid\_BatchClippingDPSGD\_client}{}
    \State \textbf{Input:} dataset (D), batch size (s), number of epochs (K), learning rate ($\eta$), Gradient norm bound (C), noise scale $\sigma$, loss function L
    %, model seed $w_0$
    \State N = len(D) \Comment{Get total number of rows in data set D}
    \State batches = divide\_dataset\_to\_batches(D,s) \Comment{detach dataset into equally data batches}
    \State B = len(batches)
    \For{batch \textbf{in} batches}
        \State normalize(batch) \Comment{Normalize data in each batch}
    \EndFor
    
    \For{$k= 0,1,2,\dots,K-1$}
        \State Wait till  current global model $\hat{w}$ is received from  Server
        \State $w = \hat{w}$
        
        \State batches = shuffle(batches)
        \For{$b = 0,1,2,\dots, B-1$}
            \State U = 0
            \State batch = shuffle(batches[b])
            \For{$t = 0,1,\dots, s/m-1$}
                \State $g = \frac{1}{m} \sum_{i=0}^{m-1} \nabla L(w,batch[tm+i])$
                \State $w \leftarrow  w - \eta_{kB+b} \cdot g$
                \State $U \leftarrow U + g$
            \EndFor
            \State $U \leftarrow [U]_C $
            %U/ \max(1,\frac{||U||_2}{C})$ 
            \Comment{Clipping gradient}
            \State $U \leftarrow U + N(0,C^2 \sigma^2 \textbf{I}) $ \Comment{Add noise to clipped gradients}
            \State Send $(kB + b, \eta_{kB+b} \cdot U)$ to the Server. 
        \EndFor
    \EndFor
\EndProcedure
\end{algorithmic}
\end{algorithm}

[TO DO: explain that individual clipping means remove clipping of $U$ and include clipping of $g$ right after $g$ is computed and no update on $w$ (no SGD)]

%%%% asynchoronous FL Hybrid Batch clipping algorithm %%%%%%
\begin{algorithm}[!ht]
\caption{Hybrid Batch Clipping DPSGD for asynchoronous Federated Learning setting}
\label{alg:fed_batch_FL_DPs}
\begin{algorithmic}[1]
%\Procedure{LocalSGDwithDP}{$d,C,s,\sigma,T$}
\Procedure{Async\_Federated\_Hybrid\_BatchClippingDPSGD\_client}{}
    \State \textbf{Input:} dataset (D), batch size (s), number of epochs (K), learning rate ($\eta$), Gradient norm bound (C), noise scale $\sigma$, loss function L
    %, model seed $w_0$
    \State N = len(D) \Comment{Get total number of rows in data set D}
    \State batches = divide\_dataset\_to\_batches(D,s) \Comment{detach dataset into equally data batches}
    \State B = len(batches)
    \For{batch \textbf{in} batches}
        \State normalize(batch) \Comment{Normalize data in each batch}
    \EndFor
%    \State \hat{w}=\hat{w}_0
    \For{$k= 0,1,2,\dots,K-1$}
%        \State Wait till  current global model $\hat{w}$ is received from  Server
        \State $w = \hat{w}$
        
        \State batches = shuffle(batches)
        \For{$b = 0,1,2,\dots, B-1$}
            \State U = 0
            \State batch = shuffle(batches[b])
            \For{$t = 0,1,\dots, s/m-1$}
                \State $g = \frac{1}{m}\sum_{i=0}^{m-1} \nabla L(w,batch[tm+i])$
                \State $w \leftarrow  w - \eta_{kB+b} \cdot g$
                \State $U \leftarrow U + g$
            \EndFor
            \State $U \leftarrow [U]_C$
            %U/ \max(1,\frac{||U||_2}{C})$ 
            \Comment{Clipping gradient}
            \State $U \leftarrow U + N(0,C^2 \sigma^2 \textbf{I}) $ \Comment{Add noise to clipped gradients}
            \State $\hat{w}\leftarrow \hat{w}+\eta_{kB+b} \cdot U$
            \State Send $(kB + b, \eta_{kB+b} \cdot U)$ to the Server. 
        \EndFor
    \EndFor
\EndProcedure

ISR replace both $w$ and $\hat{w}$ by received global model

\end{algorithmic}
\end{algorithm}
